# Supplementary material for: Preference Optimization for Reasoning with Pseudo Feedback
Source: arXiv:2411.16345 source file (2025-02-14)
Supplement: Supplementary file 1 [file prompts_text.tex]

% \begin{table}[t]
% \centering
% % \vskip 0.05in
% \renewcommand{\arraystretch}{1.4}
% \setlength{\tabcolsep}{1.2mm}{
% \scalebox{0.8}{
% \begin{tabular}{p{\linewidth}}
% \toprule
You are an expert programmer. Your task is to write some test cases to the programming problems to help verify the expected program solutions. You only need to give me the inputs in the required format. Now, let me introduce the details to you:

\#\# Program Format

There will be two kinds of programming problems. One type of problem accepts standard input-output stream. As a result, the test case inputs should contain only the inputs text stream.

Another kind of problem is based on function calling, which shows a segment of starter code to illustrate the function head, defining the name of the arguments to be accepted. In this case, you should return me the inputs in the format of function calling, like `function\_name(*arguments)`.

\#\# Response Format

You should return me the test case inputs in `json\_object` format. You need to generate **10** groups of test case inputs, and each key field is named as `test\_case\_i`, where `i` is the index of the test case. The value of each key is the test case inputs in the required format, which should be a string.

\#\# Examples for Standard Input-Output and Function Calling.

\#\#\# Standard Input-Output Stream

\#\#\#\# Programming Problem

Polycarp has $n$ different binary words. A word called binary if it contains only characters '0' and '1'. For example, these words are binary: "0001", "11", "0" and "0011100".

Polycarp wants to offer his set of $n$ binary words to play a game "words". In this game, players name words and each next word (starting from the second) must start with the last character of the previous word. The first word can be any. For example, these sequence of words can be named during the game: "0101", "1", "10", "00", "00001".

Word reversal is the operation of reversing the order of the characters. For example, the word "0111" after the reversal becomes "1110", the word "11010" after the reversal becomes "01011".

Probably, Polycarp has such a set of words that there is no way to put them in the order correspondent to the game rules. In this situation, he wants to reverse some words from his set so that:  the final set of $n$ words still contains different words (i.e. all words are unique);  there is a way to put all words of the final set of words in the order so that the final sequence of $n$ words is consistent with the game rules.

Polycarp wants to reverse minimal number of words. Please, help him.

-----Input-----

The first line of the input contains one integer $t$ ($1 \le t \le 10^4$) — the number of test cases in the input. Then $t$ test cases follow.

The first line of a test case contains one integer $n$ ($1 \le n \le 2\cdot10^5$) — the number of words in the Polycarp's set. Next $n$ lines contain these words. All of $n$ words aren't empty and contains only characters '0' and '1'. The sum of word lengths doesn't exceed $4\cdot10^6$. All words are different.

Guaranteed, that the sum of $n$ for all test cases in the input doesn't exceed $2\cdot10^5$. Also, guaranteed that the sum of word lengths for all test cases in the input doesn't exceed $4\cdot10^6$.

-----Output-----

Print answer for all of $t$ test cases in the order they appear.

If there is no answer for the test case, print -1. Otherwise, the first line of the output should contain $k$ ($0 \le k \le n$) — the minimal number of words in the set which should be reversed. The second line of the output should contain $k$ distinct integers — the indexes of the words in the set which should be reversed. Words are numerated from $1$ to $n$ in the order they appear. If $k=0$ you can skip this line (or you can print an empty line). If there are many answers you can print any of them.

-----Example-----\\
Input\\
4\\
4\\
0001\\
1000\\
0011\\
0111\\
3\\
010\\
101\\
0\\
2\\
00000\\
00001\\
4\\
01\\
001\\
0001\\
00001

Output\\
1\\
3\\
-1\\
0

2\\
1 2\\

\#\#\#\# Response

\{\\
\quad "test\_case\_0": "3$\backslash$n3$\backslash$n101$\backslash$n110$\backslash$n011$\backslash$n2$\backslash$n01$\backslash$n10$\backslash$n4$\backslash$n0001$\backslash$n1000$\backslash$n0011$\backslash$n0111",\\
\quad "test\_case\_1": "2$\backslash$n2$\backslash$n01$\backslash$n10$\backslash$n3$\backslash$n000$\backslash$n111$\backslash$n110",\\
\quad ...\\
\}

\#\#\# Function Calling

\#\#\#\# Programming Problem

Given a single positive integer x, we will write an expression of the form x (op1) x (op2) x (op3) x ... where each operator op1, op2, etc. is either addition, subtraction, multiplication, or division (+, -, *, or /).  For example, with x = 3, we might write 3 * 3 / 3 + 3 - 3 which is a value of 3.
When writing such an expression, we adhere to the following conventions:

The division operator (/) returns rational numbers.
There are no parentheses placed anywhere.
We use the usual order of operations: multiplication and division happens before addition and subtraction.
It's not allowed to use the unary negation operator (-).  For example, "x - x" is a valid expression as it only uses subtraction, but "-x + x" is not because it uses negation.

We would like to write an expression with the least number of operators such that the expression equals the given target.  Return the least number of operators used.

Example 1:

Input: x = 3, target = 19

Output: 5

Explanation: 3 * 3 + 3 * 3 + 3 / 3.  The expression contains 5 operations.

Example 2:

Input: x = 5, target = 501

Output: 8

Explanation: 5 * 5 * 5 * 5 - 5 * 5 * 5 + 5 / 5.  The expression contains 8 operations.

Example 3:

Input: x = 100, target = 100000000

Output: 3

Explanation: 100 * 100 * 100 * 100.  The expression contains 3 operations.

Note:

$2 \le x \le 100$

$1 \le target \le 2 \times 10^8$

class Solution:\\
    def leastOpsExpressTarget(self, x: int, target: int) - > int:

\#\#\#\# Response

\{\\
    "test\_case\_0": "leastOpsExpressTarget(3, 19)",\\
    "test\_case\_1": "leastOpsExpressTarget(3, 32)",\\
    "test\_case\_2": "leastOpsExpressTarget(6, 100)",\\
    ...\\
\}

\#\# Get Started

Note that in the above examples, I omit some test case inputs. You should return **10** groups of inputs to me in `json\_object` format.

\#\#\#\# Programming Problem

[[Question]]

\#\#\#\# Response
